# Supplementary material for: CONFIDE: Contextual Finite Differences Modelling of PDEs
Source: arXiv:2303.15827 source file (2024-06-07)
Supplement: Supplementary file 1 [file di.tex]

\textbf{Direct Identification (DI).}
We used this rather simple algorithm as a measuring tool to evaluate the abilities of PDExplain to recover the correct coefficients when they are constants.
The algorithm simply searches for the coefficients that provides the best numerical solution for the PDE, for each of the test signals.
Note, that this is not a learning algorithm but an inference algorithm for directly identifying the coefficients of the PDE.
The numerical solution is evaluated in the same way as PDExplain, and the coefficients are searched via gradient descent in the coefficient space using \verb|pyTorch| automatic differentiation.
This is done by manually setting the coefficient vector to an initial value $p_0$, and gradually converging in the direction of the coefficients that best solve the PDE.
To evade local-minima we start from several different initial value locations in the coefficient space, and keep the coefficients that achieve lowest loss per signal.
In the only experiment where DI can be used, the constant coefficients second order PDE, the loss is evaluated by:
\begin{align*}
    \mathop{\min}\limits_{a,b,c}\left\Vert \fder{u}{t} - \hat{a} \cdot \sder{u}{x} - \hat{b} \cdot \fder{u}{x} - \hat{c} \right\Vert,
\end{align*}
where the parameters are computed per test signal.
An alternative approach of grid-searching the coefficients cannot be applied without directly knowing the range and scale of the coefficients.

We note that although DI has the ability to recover the closest coefficients to the ground truth, it cannot generalize from a training set to the test set.
Learning from a train set enables PDExplain to learn the range of physically feasible coefficient functions, thus avoiding an output of coefficients that result in diverging signals.
Another important note about DI, is that it cannot be directly applied for identifying a coefficient function (as in the Burgers' and FitzHugh-Nagomu equations).
