# Supplementary material for: CONFIDE: Contextual Finite Differences Modelling of PDEs
Source: arXiv:2303.15827 source file (2024-06-07)
Supplement: Supplementary file 2 [file fd_vs_integration.tex]

\label{app:FD_VS_ODE}
A key part in the CONFIDE algorithm is its use of numerical evaluation of spatio-temporal derivatives through the finite-differences approach.
As shown throughout this paper, using finite differences combined with the a-priori known mechanistic form of the PDE provides both coefficients estimation and reliable predictions.
However, there's another important advantage that a finite-differences approach has on other integral approaches (such as the adjoint method used in Neural-ODE \citep{chen2018neural} and other relevant works), the amount of time necessary for training the model.

To demonstrate this effect we create a toy example based on an ODE of a single pendulum without friction:
\begin{align*}
    \ddot{\theta} = - \frac{g}{l} \sin (\theta),
\end{align*}
where $g$ is the gravitational parameter, $\theta$ is the angle of the pendulum, and $l$ is the length of the pendulum.
We created a train set of 10,000 signals that obey the pendulum ODE, with the length parameter $l$ sampled for each signal $l\sim U[1,2]$, the initial conditions of $\theta(t=0)$ sampled from $\theta \sim U[-0.4,0.4]$ and the initial conditions of the angular velocity $\dot{\theta}=\omega\sim U[-0.1,0.1]$.

The two algorithms that are tested are CONFIDE and a version of Neural-ODE that also receives the ODE form of the pendulum.
We used the ODE-aware version of Neural-ODE so that both algorithms are presented with the same information and have the same goals: to estimate the length of the pendulum on a given signal $l$, and provide the observed signal future prediction $\theta(t>T)$, where the observation is up to time $T$.

Both algorithms use a single neural-network that consumes an observed signal, and generates an estimation $\hat{l}$.
The next step of both algorithms is to enforce that $\hat{l}$ can generate the observed signal. 
CONFIDE uses a differentiation approach by numerically evaluating the time derivative of the observed signal, and comparing this derivative to the function of the ODE. I.e., minimizing the objective:
\begin{align*}
    \min \left\Vert \frac{d^2\theta}{dt^2} - \frac{g}{\hat{l}} \sin (\theta) \right\Vert,
\end{align*}
where ${d^2\theta}/{dt^2}$ is evaluated through finite differences.
At inference time, the observation is consumed by the neural-network, which outputs $\hat{l}$. We then feed $\hat{l}$ and the initial conditions to an ODE solver to obtain the prediction.
Neural-ODE uses the initial value ($\theta(t=0)$) and $\hat{l}$ to generate the signal $\hat{\theta}(t=0,..,T)$, and compare the generated signal to the observed one using an MSE loss.
We trained both algorithms in exactly the same setting, over 5 epochs, and observed that CONFIDE train significantly faster. Specifically, CONFIDE's training time took 3.6 seconds, and neural-ODE's training time took 159.2 seconds.
I.e., \textbf{CONFIDE trained $\sim 44$ times faster than Neural-ODE}.

In figure~\ref{fig:appendix.FD_VS_ODE} and in table~\ref{tbl:experiments.all_error}, we see that not only did CONFIDE train much faster, it also was able to provide very reliable results, both in terms of prediction and in terms of parameter estimation.

\begin{figure}[H]
\centering
\includegraphics[width=0.6\textwidth]{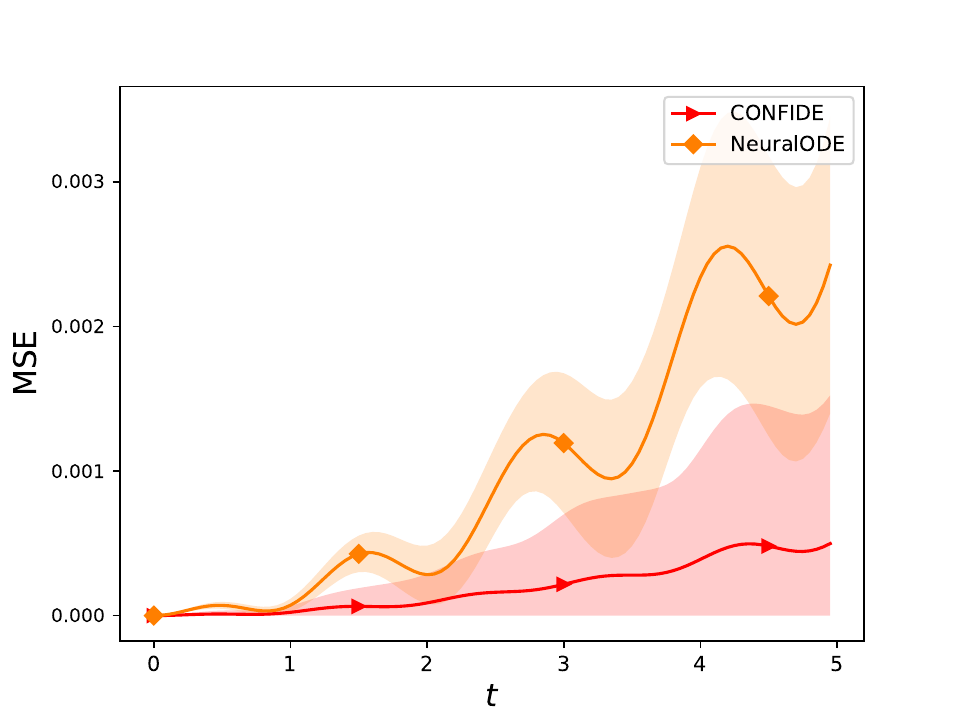}
\caption{Pendulum ODE: prediction error as horizon increases, for different approaches.}
\label{fig:appendix.FD_VS_ODE}
\end{figure}

% \begin{table}[H]
% \centering
%         \begin{tabular}{lccc}
%             \toprule
%             Algorithm & Prediction MSE & Coefficient MSE & Training time\\
%             \midrule
%             CONFIDE & $0.0002 \pm 0.0003$ & $0.1598 \pm 0.1891$ & $3.6 \text{s}$\\
%             Neural-ODE & $0.0010 \pm 0.0003$ & $0.1702 \pm 0.2021$ & $159.2s$\\
%             \bottomrule
%         \end{tabular}
% \caption{Results summary on the pendulum ODE in terms of future time prediction error, pendulum length estimation error and training time between two different approaches: a differentiation approach (CONFIDE) and an integral approach (Neural-ODE)}
% \label{tbl:experiments.all_error}
% \end{table}
