# Supplementary material for: CONFIDE: Contextual Finite Differences Modelling of PDEs
Source: arXiv:2303.15827 source file (2024-06-07)
Supplement: Supplementary file 3 [file ood.tex]

\label{app:sec.ood}
In this section, we provide additional experiments conducted on out-of-distribution (OOD) data. 
These experiments where selected to demonstrate how CONFIDE can handle observations that are significantly different than the data in the train set.
We divide the OOD experiments into two parts: (1) the initial conditions observed are not smooth and have some discontinuity, and (2) the parameters used to generate the signals in the test set are sampled from a different distribution than the one used in the train set.

\label{app:ood.1}
\subsection{Non-smooth initial conditions}
Continuing the discussion in the paper, we demonstrate how CONFIDE handles the case where the observed data has a non smooth point.
% Testing CONFIDE on non-smooth signals is important mainly because in this method we evaluate the spatio-temporal derivatives of the signal numerically using a finite-differences approach.
% This computation might result in very high derivatives in these non-smooth locations and interfere with the optimization task.
% Although CONFIDE was not designed specifically for this task, a straight-forward solution would be to evaluate if the observed signal has non-smooth locations, and to not include the derivatives evaluated in these locations in the optimization task. For example, if $u(t=0, x=L/2)$ is non-smooth, then the optimization task defined in equation~\ref{eq:coefficient_estimator_loss} will be performed on the smooth parts separately and summed together.
% We note that in this test we did not use the above solution since the goal is to test CONFIDE's capabilities in its vanilla form.

For this benchmark, we generated a new test set based on the Burgers' equation experiment, where the initial conditions are not sampled from a single Gaussian process (as described in section~\ref{app:implementation}), but from two distinct Gaussian processes. 
The first Gaussian process sampled serves as the left part of the initial condition ($x=0,..,L/2$) and obeys $u(t=0,x=0)=u(t=0,x=L/2)=0$, and the second Gaussian process sampled serves as the right part of the initial condition ($x=L/2,...,L$) and obeys $u(t=0,x=L/2)=1,  u(t=0,x=L)=0$.
This formulation creates a discontinuity in the initial conditions at $x=L/2$.
We generated 1000 test-signals, all sharing the same characteristics as the Burgers' equations experiment, except all of them have a discontinuity at $u(t=0,x=L/2)$. 
In figure~\ref{app:shockwave_demo} we demonstrate two initial conditions of shock-wave signals from the test set.
% We stress that the train-set is still the original one, since our goal is to  test whether CONFIDE is able to handle OOD data, which, in this case, comes in the form of OOD initial conditions.

\begin{figure}
    \centering
    \begin{subfigure}[b]{0.49\textwidth}
        \includegraphics[width=\textwidth]{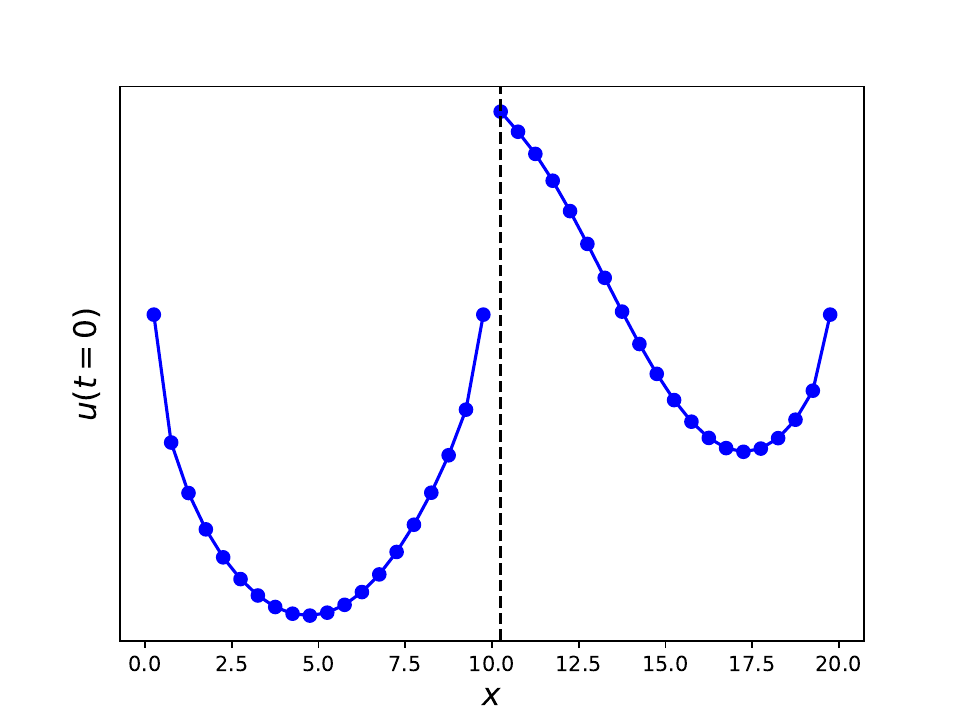}
        \caption{}
        \label{app:shockwave_demo_1}
    \end{subfigure}
    \centering
    \begin{subfigure}[b]{0.49\textwidth}
        \includegraphics[width=\textwidth]{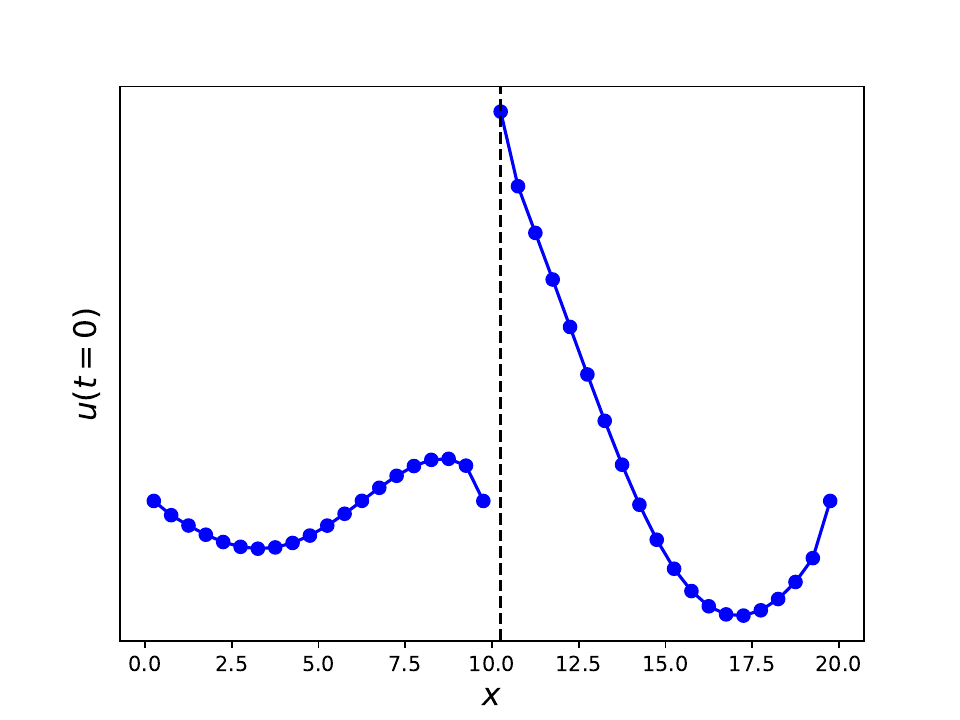}
        \caption{}
        \label{app:shockwave_demo_2}
    \end{subfigure}
    \caption{Demonstration of two initial conditions of shock-wave signals from the test set. Both signals have a discontinuity in $x=L/2$ (for $L=20$).}
    \label{app:shockwave_demo}
\end{figure}

As shown in figure~\ref{app:shockwave}, CONFIDE successfully predicts the given observations and outperforms other baselines, even when it never observed such signals in the train set.
The reason is that CONFIDE evaluates the derivatives at different times of the observed context $u^c$ at each iteration, and most of them are smooth.

\label{app:ood.2}
\subsection{OOD coefficients}
In the second benchmark, we continuing the discussion in the paper, and demonstrate how CONFIDE handles the case where the observed signal in the test set is generated from a PDE with coefficients that come from different distribution than the ones in the train set.

For this benchmark, we generated a new test set based on the Burgers' equation experiment, where the coefficient $a$ is sampled from $u\sim U[2,4]$ instead of  $u\sim U[1,2]$ as in the train set. 
This modification in the coefficients distribution, results in generated signals that might be significantly different than the ones observed in the train set.
As shown in figure~\ref{app:ood_coeff}, CONFIDE successfully predicts the observed signal, and outperforms other baselines.
% We note that since CONFIDE learns to output coefficients only in the range of the coefficients in the train set, it projects the observed signal to the range of coefficients in the train set so that it best describes the observed signal.

\begin{figure}
    \centering
    \begin{subfigure}[b]{0.49\textwidth}
        \includegraphics[width=\textwidth]{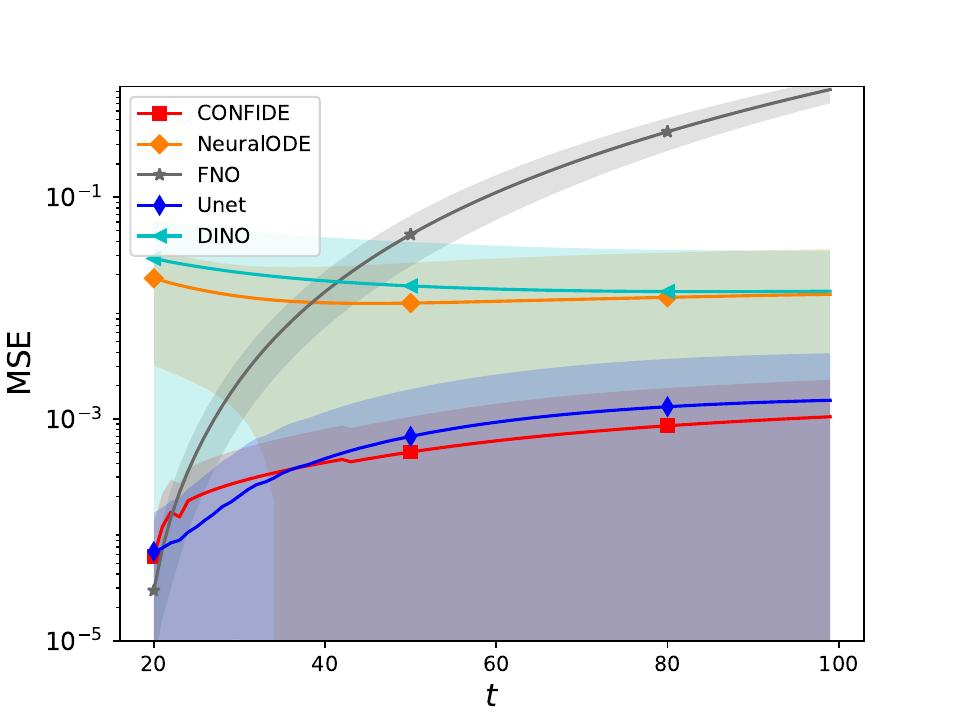}
        \caption{}
        \label{app:shockwave}
    \end{subfigure}
    \centering
    \begin{subfigure}[b]{0.49\textwidth}
        \includegraphics[width=\textwidth]{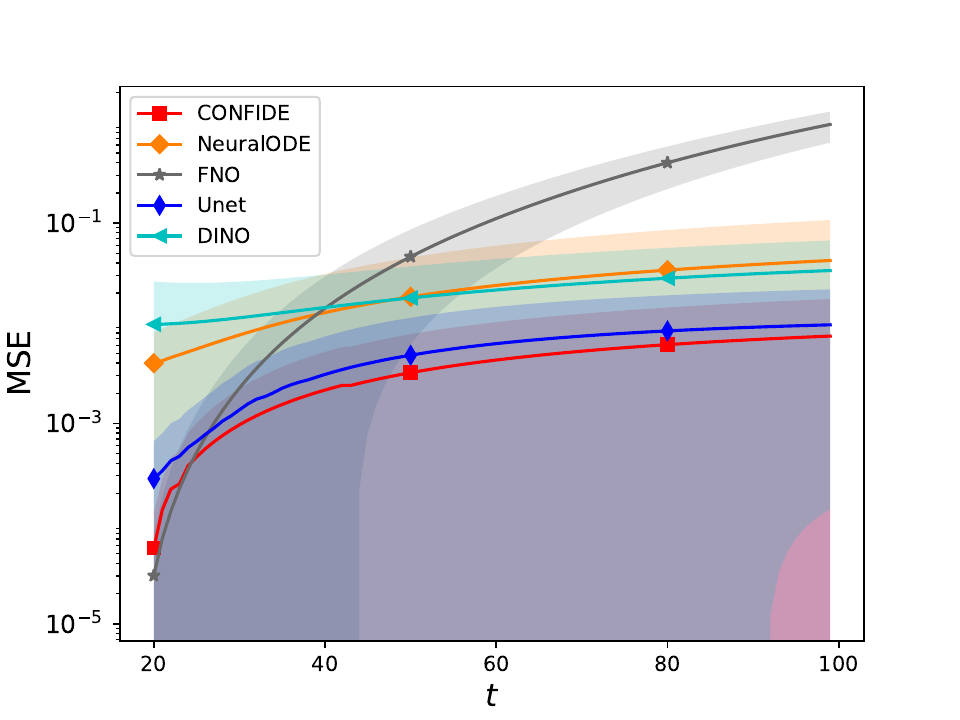}
        \caption{}
        \label{app:ood_coeff}
    \end{subfigure}
    \caption{Prediction error as horizon increases on the two OOD benchmarks for different approaches. In (a) we show prediction results of all approaches on test set that includes a discontinuity in the initial conditions (shock-wave), and in (b) we show prediction results on OOD coefficients (I.e., test set generated from coefficients from different distribution than the ones used in the train set).}
\end{figure}

% \begin{table}[H]
% \centering
%         \begin{tabular}{lcc}
%             \toprule
%             Algorithm & \shortstack{Prediction MSE \\ shock-wave} & \shortstack{Prediction MSE \\ OOD coefficients}\\
%             \midrule
%     CONFIDE & $0.0010 \pm 0.0012$ & $0.0074 \pm 0.0100$\\
%     Neural-ODE & $0.0133 \pm 0.0208$ & $0.0423 \pm 0.0649$\\
%     FNO & $0.9367 \pm 0.2322$ & $0.9646 \pm 0.3304$\\
%     Unet & $0.0015 \pm 0.0024$ & $0.0096 \pm 0.0121$\\
%                 \bottomrule
%         \end{tabular}
% \caption{Results summary on the two OOD benchmarks for different approaches.}
% \label{tbl:app_ood}
% \end{table}
